# Supplementary material for: Towards Instance-Optimality in Online PAC Reinforcement Learning
Source: arXiv:2311.05638 source file (2023-10-31)
Supplement: Supplementary file 1 [file app_EDIPE.tex]

\section{Analysis of EDIPE}
\subsection{Good event}
We define the events
\begin{align*}
    \cE_{r} &:= \bigg(\forall k \in \mathbb{N}^\star\ \forall \pi \in \PiS,\ \bigg|\sum_{h,s,a}  p_h^{\pi}(s,a)\Big(\widehat{r}_h^{k}(s,a) - r_h(s,a)\Big) \bigg| \leq \sqrt{\beta^{bpi}(t_k,\delta/3)\sum_{h,s,a}\frac{p_h^{\pi}(s,a)^2}{n_h^k(s,a)}} \bigg)\\
    \cE_{cnts} &:= \bigg(\forall t\geq t_0 \ \forall (h,s,a),\  n_h^t(s,a) - n_h^{0}(s,a)\geq \frac{\overline{n}_h^t(s,a)- \overline{n}_h^{0}(s,a)}{2} - \log(3SAH/\delta) \bigg)\\
    \cE_{cov} &:= \bigg(\textrm{CovGame run with inputs $(c^{0}, \delta/3)$ terminates after at most}\\
    & 64 m_0 \varphi^\star(c^{0}) + \widetilde{\cO}\big(m_0 \varphi^\star(\mathds{1}) SAH^2 (\log(3/\delta) + S) \big)\ \textrm{episodes and returns a dataset $\cD_0$ }\\
    &\textrm{such that for all } (h,s,a), n_h(s,a;\cD_0)\geq c^{0}_h(s,a) \bigg),
\end{align*}
where $m_0 = \log_2\big(\frac{\max_{s,a,h} c_h^{0}(s,a)}{\min_{s,a,h} c_h^{0}(s,a) \vee 1}\big) \vee 1$ and $\beta^{bpi}$ is defined in appendix \ref{sec:app-concentration-RFE}. Then our good event is defined as the intersection 
\begin{align*}
    \cE_{good} :=  \cE_{r} \cap \cE_{cnts} \cap \cE_{cov}.
\end{align*}

\subsection{Optimal policies are never eliminated}
\begin{lemma}\label{lem:optimal-never-eliminated}
    Under the good event, for all policies $\pi^\star \in \Pi^\star$ and all phases $k\geq 0$, it holds that at the end of phase $k$, $p^{\pi^\star} \in \Omega^k$.  
\end{lemma}
\begin{proof}
We fix an optimal policy $\pi^\star$ and prove the statement by induction. For $k=0$ the fact that ${p}^{\pi^\star} \in \Omega^0$ is trivial, since $\Omega^0 = \Omega$ consists of all state-action distributions that are valid under the transition kernel ${p}$. Now suppose that the property holds at the end of phase $k-1$. We first show that $\sum_{h,s,a} \frac{p_h^{\pi^\star}(s,a)^2}{n_h^{k}(s,a)} \leq 2^{-k}$. To that end, let us write
\begin{align*}
    \sum_{h,s,a} \frac{p_h^{\pi^\star}(s,a)^2}{n_h^{k}(s,a)} &{\leq} \sum_{h,s,a} \frac{p_h^{\pi^\star}(s,a)^2}{ n_h^{0}(s,a) + \big[\overline{n}_h^{t_k}(s,a) - \overline{n}_h^{t_0}(s,a) \big]/2 - \log(3SAH/\delta)} \tag{by event $\cE_{cnt}$}\\
    &{\leq} 2\sum_{h,s,a} \frac{p_h^{\pi^\star}(s,a)^2}{\overline{n}_h^{t_k}(s,a) - \overline{n}_h^{t_0}(s,a)} \tag{by event $\cE_{cov}$} \\
    &{\leq} 2\sum_{h,s,a} \frac{p_h^{\pi^\star}(s,a)^2}{d_k p^{\pi^{k}}_h(s,a)} \tag{by def of the phases $\overline{n}_h^{t_k}(s,a) - \overline{n}_h^{t_0}(s,a) = \sum\limits_{j=1}^k d_j p^{\pi^j}_h(s,a)$ }\\
    &{\leq} 2 \max_{\rho\in \Omega^{k-1}}\sum_{h,s,a} \frac{\rho_h(s,a)^2}{d_k p^{\pi^{k}}_h(s,a)} \tag{by induction hypothesis}\\
    &=  2\frac{E^\star_k}{\left\lceil 2^{k+1} E^\star_k \right\rceil} \tag{by def of $\pi^k$ and $d_k$}\\
    &\leq 2^{-k}.
\end{align*}
Now let 
\begin{align*}
    \widetilde{\rho} \in \argmax_{\substack{\rho \in \Omega,\\ \textstyle{\sum\limits_{h,s,a} \frac{\rho_h(s,a)^2}{n_h^{k}(s,a)} \leq 2^{-k}}}} \rho^\top \widehat{r}^{k}
\end{align*}
and consider any policy $\widetilde{\pi}$ whose state-action distribution is $\widetilde{\rho}$. Under the good event we have,
\begin{align*}
    (p^{\pi^\star})^\top \widehat{r}^{k} - \underline{V}_1^{k} &= (p^{\pi^\star})^\top (\widehat{r}^{k} - r) - \widetilde{\rho}^\top (\widehat{r}^{k} - r) + \big[V_1^{\pi^\star} - V_1^{\widetilde{\pi}} \big] + \sqrt{2^{1-k}\beta^{r}(t_{k},\delta/3)} \tag{definition of $\underline{V}_1^{k}$ and $\widetilde{\pi}$}\\
    &{\geq} \sqrt{2^{2-k}\beta^{r}(t_{k},\delta/3)} - \sqrt{\beta^r(t_k,\delta/3) \sum_{h,s,a} \frac{p_h^{\pi^\star}(s,a)^2}{n_h^{t_k}(s,a)}} - \sqrt{\beta^r(t_k,\delta/3) \sum_{h,s,a} \frac{p_h^{\widetilde{\pi}}(s,a)^2}{n_h^{t_k}(s,a)}} \tag{by event $\cE_r$}\\
    &= \sqrt{2^{2-k}\beta^{r}(t_{k},\delta/3)} - \sqrt{\beta^r(t_k,\delta/3) \sum_{h,s,a} \frac{p_h^{\pi^\star}(s,a)^2}{n_h^{t_k}(s,a)}} -  \sqrt{\beta^r(t_k,\delta/3)\sum\limits_{h,s,a} \frac{\widetilde{\rho}_h(s,a)^2}{n_h^{k}(s,a)}} \\
    &\geq \sqrt{2^{2-k}\beta^{r}(t_{k},\delta/3)} - 2\sqrt{2^{-k}\beta^{r}(t_{k},\delta/3)} \tag{by def of $\widetilde{\rho}$ and the inequality above}\\
    &= 0.
\end{align*}
Hence we just proved that $p^{\pi^\star}$ is in $\Omega^k$.
\end{proof}

\subsection{Correctness}
\begin{lemma}
    Suppose that EDIPE stops and let $\widehat{\pi}$ be the policy that it returns. Then 
    $$\bP_{\cM}\left(V_1^{\widehat{\pi}} \geq V_1^\star - \epsilon\right) \geq 1-\delta.$$
    In other words, EDIPE is $(\epsilon, \delta)$-PAC.
\end{lemma}
    
\begin{proof}
Assume that EDIPE stops as phase $k$ and let $\widehat{r}^k$ denote the empirical estimate of the mean-reward vector at the end of that phase. By definition $\widehat{\pi}$ is the policy corresponding to $\widehat{\rho}^\star \in \argmax_{\rho \in \Omega^{k}} \rho^\top \widehat{r}^{k}$. Therefore under the good event we have
\begin{align*}
    V_1^{\widehat{\pi}} &= (\widehat{\rho}^\star)^\top r\\
    &{\geq} (\widehat{\rho}^\star)^\top \widehat{r}^{k} - \sqrt{\beta^{bpi}(t_{k},\delta/3) \sum_{h,s,a}\frac{\widehat{\rho}^\star_h(s,a)^2}{n_h^{k}(s,a)}} \tag{by event $\cE_r$}\\
    & {\geq} (p^{\pi^\star})^\top \widehat{r}^{k} -  \sqrt{\beta^{bpi}(t_{k},\delta/3) \sum_{h,s,a}\frac{\widehat{\rho}^\star_h(s,a)^2}{n_h^{k}(s,a)}} \tag{def of $\widehat{\rho}^\star$}\\
    &{\geq} ({p}^{\pi^\star})^\top r - \sqrt{\beta^{bpi}(t_{k},\delta/3) \sum_{h,s,a}\frac{p^{\pi^\star}_h(s,a)^2}{n_h^{k}(s,a)}} - \sqrt{\beta^{bpi}(t_{k},\delta/3) \sum_{h,s,a}\frac{\widehat{\rho}^\star_h(s,a)^2}{n_h^{k}(s,a)}} \tag{by event $\cE_r$}\\
    &{\geq} V_1^\star - 2\sqrt{\beta^{bpi}(t_{k},\delta/3)2^{-k}} \tag{by Lemma \ref{lem:optimal-never-eliminated} and def of $\widehat{\rho}^\star$} \\
    &{\geq} V_1^\star - \epsilon \tag{by the stopping condition}.
\end{align*}

\end{proof}

\subsection{Upper bound on final phase}
\begin{lemma}\label{lem:EDIPE-final-phase}
Define the index of the final phase of EDIPE, $\kappa_f := \inf \big\{k\in \bN_{+}: \sqrt{\beta^{bpi}(t_{k},\delta/3)2^{2-k}} \leq \epsilon \big\}$. Further let $\tau$ denote the number of episodes played by the algorithm. Then under the good event, it holds that $\kappa_f < \infty$ and
\begin{align*}
     2^{\kappa_f} \leq \frac{8\beta^{bpi}(\tau,\delta/3)}{\epsilon^2}.
\end{align*}
\end{lemma}
\begin{proof}
First we prove that $\kappa_f$ is finite. Under the good event we have
\begin{align*}
    t_k &= \sum_{j=0}^k d_j\nonumber\\    
    &= d_0+ \sum_{j=0}^k 2^{j+1}\underset{\eta\in\Omega}{\min} \max_{\rho\in \Omega^{j-1}}\sum_{h,s,a} \frac{\rho_h(s,a)^2}{\eta_h(s,a)}\\
    &\leq d_0 + 2^{k+2}\underset{\eta\in\Omega}{\min} \max_{\rho\in \Omega}\sum_{h,s,a} \frac{\rho_h(s,a)^2}{\eta_h(s,a)} \tag{$\Omega^{j-1}\subset \Omega$}.
\end{align*}
On the other hand
\begin{align}\label{eq:bound_d_0}
    d_0 &\leq 64 m_0 \phi^\star([\log(3SAH/\delta)]_{h,s,a}) + \widetilde{\cO}\big(m_0 \varphi^\star(\mathds{1}) SAH^2 (\log(3/\delta) + S) \big)\quad \textrm{(by event $\cE_{cov}$)} \nonumber\\
    &= 64m_0\log(3SAH/\delta) \varphi^\star(\mathds{1}) + \widetilde{\cO}\big(m_0 \varphi^\star(\mathds{1}) SAH^2 (\log(3/\delta) + S) \big)\quad \textrm{($\phi^\star(\alpha c) = \alpha \phi^\star(c)$ by Lemma something in the colt paper)} \nonumber\\
    &= \widetilde{\cO}\big(\varphi^\star(\mathds{1}) SAH^2 (\log(3/\delta) + S) \big),
\end{align}
where we recall that $m_0 = \log_2\big(\frac{\max_{s,a,h} c_h^{0}(s,a)}{\min_{s,a,h} c_h^{0}(s,a) \vee 1}\big) \vee 1 = 1$ because $c_h^0(s,a) = \log(3SAH/\delta)$ for all $(h,s,a)$. Therefore 
\begin{align}\label{ineq:final-phase-finite-1}
  t_k &= \cO_{k\to\infty}\big( 2^k \big).
\end{align}
Now recall that the threshold $\beta^{bpi}$ was defined in Appendix \ref{sec:app_concentration} as
\begin{align}\label{ineq:final-phase-finite-2}
    \beta^{bpi}(t,\delta) = 4H^2\log(1/\delta) + 24SAH^3\log(1+ t)
\end{align}
Combining (\ref{ineq:final-phase-finite-1}) and (\ref{ineq:final-phase-finite-2}) gives that 
\begin{align*}
   \beta^{bpi}(t_{k},\delta/3) = o_{k\to\infty}\big(2^k\big).
\end{align*}
Therefore $\kappa_f = \inf \big\{k\in \bN_{+}: \sqrt{\beta^{bpi}(t_{k},\delta/3)2^{2-k}} \leq \epsilon \big\}$ is indeed finite. The proof of the second statement is straightforward by noting that $\kappa_f-1$ does not satisfy the stopping condition (Line 15 in Algorithm \ref{alg:EDIPE}) and using the (crude) upper bound $t_{\kappa_f-1} \leq \tau$.
\end{proof}

\subsection{Upper bound on phases where a suboptimal policy is active}

\begin{lemma}\label{lem:EDIPE-elimination-phase}
Let $\pi$ be any suboptimal policy and $k$ such that EDIPE did not stop at phase $k$ and ${p}^{\pi} \in \Omega^k$. Further let $\tau$ denote the number of episodes played by the algorithm. Then under the good event, we have the inequality
\begin{align*}
        2^{k} \leq \frac{16\beta^{bpi}(\tau,\delta/3)}{\max(\epsilon, \Delta(\pi))^2},
\end{align*}
where $\Delta(\pi) := V_1^\star(s_1 ; r) - V_1^{\pi}(s_1 ; r)$ denotes the policy gap of $\pi$.
\end{lemma}
\begin{proof}
Let $\pi^\star$ be any optimal policy. Then we have
\begin{align*}
    V_1^\star - \sqrt{\beta^{bpi}(t_k,\delta/3) \sum_{s,a,h}\frac{p^{\pi^\star}_h(s,a)^2}{n_h^{k}(s,a)}} &{\leq} (p^{\pi^\star})^\top \widehat{r}^{k} \tag{by event $\cE_r$} \\
    &{\leq}  \sup_{\substack{\rho \in \Omega,\\ \textstyle{\sum\limits_{h,s,a} \frac{\rho_h(s,a)^2}{n_h^{k}(s,a)} \leq 2^{-k}}}} \rho^\top \widehat{r}^{k} \tag{by Lemma \ref{lem:optimal-never-eliminated}} \\ 
    &= \underline{V}_1^{\star, k} + \sqrt{2^{2-k}\beta^{bpi}(t_k,\delta/3)}\\
    &{\leq} ({p}^{\pi})^\top \widehat{r}^{k} + \sqrt{2^{2-k}\beta^{bpi}(t_k,\delta/3)}\tag{since ${p}^{\pi} \in \Omega^k$}\\
    &{\leq} V_1^\pi + \sqrt{\beta^{bpi}(t_k,\delta/3) \sum_{s,a,h}\frac{{p}^{\pi,}_h(s,a)^2}{n_h^{k}(s,a)}}+ \sqrt{2^{2-k}\beta^{bpi}(t_k,\delta/3)}.
\end{align*}
Rewriting the inequality above we get that
\begin{align}\label{ineq:elimination-PRINCIPLE}
    \Delta(\pi) &= V_1^{\star} - V_1^\pi \nonumber\\
    &\leq \sqrt{\beta^{bpi}(t_k,\delta/3) \sum_{s,a,h}\frac{\widehat{p}^{\pi^\star,k}_h(s,a)^2}{n_h^{k}(s,a)}} + \sqrt{\beta^{bpi}(t_k,\delta/3) \sum_{s,a,h}\frac{\widehat{p}^{\pi,k}_h(s,a)^2}{n_h^{k}(s,a)}}+ \sqrt{2^{2-k}\beta^{bpi}(t_k,\delta/3)} \nonumber\\
    &\leq 2\sqrt{2^{-k}\beta^{bpi}(t_k,\delta/3)} + \sqrt{2^{2-k}\beta^{bpi}(t_k,\delta/3)} = 4\sqrt{2^{-k}\beta^{bpi}(t_k,\delta/3)}. \tag{since both ${p}^{\pi^\star}$ and ${p}^{\pi}$ are in $\Omega^k$}
\end{align}

Therefore, using a crude bound $t_k \leq \tau$ we get that
\begin{align*}
    2^{k} \leq  \frac{16\beta^{bpi}(\tau,\delta/3)}{\Delta(\pi)^2}.
\end{align*}
Combining the result above with Lemma \ref{lem:EDIPE-final-phase} and the fact that $k \leq \kappa_f$ yields the final result.
\end{proof}

\subsection{Proof of Theorem \ref{thm:EDIPE-complexity}}
\begin{proof}
We write
\begin{align*}
    \tau &= \sum_{k=0}^{\kappa_f} d_k\\
    &= d_0 + \sum_{k=1}^{\kappa_f} \left\lceil 2^{k+1} E^\star_k \right\rceil\\
    &\leq d_0 + \sum_{k=1}^{\kappa_f}  2^{k+2}  \underset{\eta\in\Omega}{\min} \max_{\rho\in \Omega^{k-1}}\sum_{h,s,a} \frac{\rho_h(s,a)^2}{\eta_h(s,a)} \tag{$\lceil x \rceil \leq 2x$ for $x\ge 1$} \\
    &= d_0 + \sum_{k=1}^{\kappa_f}  2^{k+2} \underset{\eta\in\Omega}{\min}\max_{\rho\in \Omega} \mathds{1}(\rho\in \Omega^{k-1})\sum_{h,s,a} \frac{\rho_h(s,a)^2}{\eta_h(s,a)}\\
    &= d_0 + 4\sum_{k=1}^{\kappa_f}   \underset{\eta\in\Omega}{\min}\max_{\pi\in\PiS} 2^{k}\mathds{1}(p^{\pi}\in \Omega^{k-1})\sum_{h,s,a} \frac{p^{\pi}_h(s,a)^2}{\eta_h(s,a)} \tag{every $\rho\in\Omega$ corresponds to a stochastic policy $\pi\in\PiS$ and vice versa}\\
    &\leq d_0 + 4 \sum_{k=1}^{\kappa_f} \underset{\eta\in\Omega}{\min}\max_{\pi\in\PiS} \sum_{h,s,a} \frac{16 \beta^{bpi}(\tau,\delta/3) p^{\pi}_h(s,a)^2}{\eta_h(s,a)\max(\epsilon, \Delta(\pi))^2 }\tag{by Lemma \ref{lem:EDIPE-elimination-phase}}\\
    &\leq  \widetilde{\cO}\big(\varphi^\star(\mathds{1}) SAH^2 (\log(3/\delta) + S) \big)  +64 \beta^{bpi}(\tau,\delta/3) \kappa_f \underset{\eta\in\Omega}{\min}\max_{\pi\in\PiS}\sum_{h,s,a} \frac{p^{\pi}_h(s,a)^2}{\eta_h(s,a)\max(\epsilon, \Delta(\pi))^2} \tag{by inequality (\ref{eq:bound_d_0})}\\
    &\leq \widetilde{\cO}\big(\varphi^\star(\mathds{1}) SAH^2 (\log(3/\delta) + S) \big)  +64 \beta^{bpi}(\tau,\delta/3) \log_2\bigg(\frac{8\beta^{bpi}(\tau,\delta/3)}{\epsilon^2}\bigg) \underset{\eta\in\Omega}{\min}\max_{\pi\in\PiS}\sum_{h,s,a} \frac{p^{\pi}_h(s,a)^2}{\eta_h(s,a)\max(\epsilon, \Delta(\pi))^2} \tag{by Lemma \ref{lem:EDIPE-final-phase}}
\end{align*}
Combining the inequality above with the expression of the threshold $\beta^{bpi}(t,\delta) = 4H^2\log(1/\delta) + 24SAH^3\log(1+ t)$ and solving for $\tau$ yield that 
\begin{align*}
    \tau \leq \widetilde{\cO}\bigg( \big(H^2\log(1/\delta) + SAH^3\big)\underset{\eta\in\Omega}{\min}\max_{\pi\in\PiS}\sum_{h,s,a} \frac{p^{\pi}_h(s,a)^2}{\eta_h(s,a)\max(\epsilon, \Delta(\pi))^2} +\varphi^\star(\mathds{1}) SAH^2 (\log(3/\delta) + S) \bigg). 
\end{align*}
Applying Proposition \ref{prop:simplifying-complexity} finishes the proof.
\end{proof}

\subsection{Simplifying the complexity term}
\begin{proposition}\label{prop:simplifying-complexity}
 It holds that
 \begin{align*}
    \underset{\eta\in\Omega}{\min}\max_{\pi\in\red{\PiS}}\sum_{h,s,a} \frac{p^{\pi}_h(s,a)^2}{\eta_h(s,a)\max(\epsilon, \Delta(\pi))^2}\leq 4  \underset{\eta\in\Omega}{\min} \max_{\pi\in\blue{\PiD}}\sum_{h,s,a} \frac{p^{\pi}_h(s,a)^2}{\eta_h(s,a)\max(\epsilon, \Delta(\pi))^2}
 \end{align*} 
\end{proposition}
\begin{proof}
First of all, note that 
\begin{align}\label{ineq:simplifying-complexity-1}
    \underset{\eta\in\Omega}{\min}\max_{\pi\in\PiS}\sum_{h,s,a} \frac{p^{\pi}_h(s,a)^2}{\eta_h(s,a)\max(\epsilon, \Delta(\pi))^2}& \leq 4\underset{\eta\in\Omega}{\min}\max_{\pi\in\PiS}\sum_{h,s,a} \frac{p^{\pi}_h(s,a)^2}{\eta_h(s,a)(\epsilon + \Delta(\pi))^2} \nonumber\\
    &=  4\underset{\eta\in\Omega}{\min}\max_{\pi\in\PiS}\sum_{h,s,a} \frac{p^{\pi}_h(s,a)^2}{\eta_h(s,a)(\epsilon + (p^{\pi^\star} - p^{\pi})^\top r )^2}, 
\end{align}
where we used that $\Delta(\pi) = V_1^\star - V_1^\pi = (p^{\pi^\star} - p^{\pi})^\top r$. Now fix $\eta\in \Omega$. We will show that the function 
$$f: p^{\pi} \mapsto \sum_{h,s,a}\frac{p^{\pi}_h(s,a)^2}{\eta_h(s,a)(\epsilon + (p^{\pi^\star} - p^{\pi})^\top r )^2}$$
 is quasi-convex. Let $\pi^1, \pi^2$ be two policies and $\alpha\in (0,1)$. We have
\begin{align*}
  f\big((1-\alpha)p^{\pi^1} + \alpha p^{\pi^2}\big) &=  \sum_{h,s,a} \frac{\big((1-\alpha)p^{\pi^1}_h(s,a) + \alpha p^{\pi^2}_h(s,a)\big)^2}{\eta_h(s,a)(\epsilon + (p^{\pi^\star} - (1-\alpha)p^{\pi^1} - \alpha p^{\pi^2})^\top r )^2}\\
  &= \sum_{h,s,a} \frac{\bigg((1-\alpha)(\epsilon + \Delta(\pi^1))\frac{p^{\pi^1}_h(s,a)}{(\epsilon + \Delta(\pi^1))} + \alpha (\epsilon + \Delta(\pi^2)) \frac{p^{\pi^2}_h(s,a)}{(\epsilon + \Delta(\pi^2))}\bigg)^2}{\eta_h(s,a)\bigg((1-\alpha)(\epsilon + \Delta(\pi^1)) + \alpha (\epsilon + \Delta(\pi^2)) \bigg)^2}\\
  &= \sum_{h,s,a} \frac{1}{\eta_h(s,a)}\bigg((1-\lambda)\frac{p^{\pi^1}_h(s,a)}{(\epsilon + \Delta(\pi^1))} + \lambda \frac{p^{\pi^2}_h(s,a)}{(\epsilon + \Delta(\pi^2))}\bigg)^2 \tag{ for $\lambda := \frac{\alpha (\epsilon + \Delta(\pi^2))}{(1-\alpha)(\epsilon + \Delta(\pi^1)) + \alpha (\epsilon + \Delta(\pi^2))}$}\\
  &\leq  \sum_{h,s,a}  \frac{1}{\eta_h(s,a)} \bigg((1-\lambda) \frac{p^{\pi^1}_h(s,a)^2}{(\epsilon + \Delta(\pi^1))^2} + \lambda \frac{p^{\pi^2}_h(s,a)^2}{(\epsilon + \Delta(\pi^2))^2} \bigg) \tag{covexity of $x\mapsto x^2$}\\
  &= (1-\lambda)f(p^{\pi^1}) + \lambda f(p^{\pi^2}) \\
  &\leq \max(f(p^{\pi^1}), f(p^{\pi^2})).
\end{align*}
Now, thanks to Theorem 3.4.8 in \cite{Kallenberg1984LinearPA}, we know that $\{p^\pi:\ \pi\in\PiS \}$ is the convex hull of $\{p^\pi:\ \pi\in\PiD \}$. Therefore, given the quasi-convexity of $f$ we have that 
\begin{align}\label{ineq:simplifying-complexity-2}
    \max_{\pi\in\PiS}\sum_{h,s,a} \frac{p^{\pi}_h(s,a)^2}{\eta_h(s,a)(\epsilon + \Delta(\pi))^2}  & = \max_{p^\pi:\ \pi\in\PiS} f(p^{\pi})\nonumber\\
    &\leq \max_{p^\pi:\ \pi\in\PiD} f(p^{\pi}) \nonumber\\
    &= \max_{\pi\in\PiD}\sum_{h,s,a} \frac{p^{\pi}_h(s,a)^2}{\eta_h(s,a)(\epsilon+ \Delta(\pi))^2}\nonumber\\
    &\leq  \max_{\pi\in\PiD}\sum_{h,s,a} \frac{p^{\pi}_h(s,a)^2}{\eta_h(s,a)\max(\epsilon, \Delta(\pi))^2}.
\end{align}
Combining (\ref{ineq:simplifying-complexity-1}) and (\ref{ineq:simplifying-complexity-2}) finishes the proof.
\end{proof}
