# Supplementary material for: Towards Instance-Optimality in Online PAC Reinforcement Learning
Source: arXiv:2311.05638 source file (2023-10-31)
Supplement: Supplementary file 2 [file app_experimental_design.tex]

\section{Experimental design properties}

\begin{algorithm}[h]
    \caption{MinFlow (for with known transitions)}\label{alg:static-cov}
    \begin{algorithmic}[1]
    \STATE \textbf{Input: } target function $c: [H]\times\cS\times\cA \to \mathbb{R}_{+}$, Transition kernels $[p_h(.|s,a)]_{h,s,a}$
    
    \STATE Solve 
        \begin{align*}
            \min_{\substack{\eta \in \Omega\\
            \forall (h,s,a),\ \eta_h(s,a) \geq c_h(s,a)}}\ \sum_{a\in\cA_1} \eta_1(s_1,a)
        \end{align*}
     to get the optimal flow $(\eta^\star)_{h\in [H],s\in \cS,a\in \cA}$ and its value $\varphi^\star(c)$.
    \STATE  Set $\Tilde{\pi}^{cov} \leftarrow \Tilde{\pi}^{cov, k}$ where  
    \begin{align*}
       \forall (h,s,a),\quad   \Tilde{\pi}_h^{cov, k}(a |s) := \begin{cases}
     \frac{\eta_h^k(s,a)}{\sum_{b\in\cA_h(s)}\eta_h^k(s,b)} \quad \textrm{if} \sum_{b\in\cA_h(s)}\eta_h^k(s,b) > 0,\\
     \frac{1}{A}\quad\quad\quad\quad\quad\quad \textrm{Otherwise}
    \end{cases}  
    \end{align*}
    \STATE Set $d \leftarrow \left\lceil \varphi^\star(c^k) \right\rceil$
    \STATE Play $\Tilde{\pi}^{cov}$ for $d$ episodes
    \STATE \textbf{return} $d$
    \end{algorithmic}
    \end{algorithm}

\begin{lemma}\label{lem:static-minflow-coverage}
    Let $c: [H]\times\cS\times\cA \to \mathbb{R}$ be a target function such that $\varphi^\star(c)$ is finite. Assume that at the end of episode $t_{start} \in \mathbb{N}$ we call the MinFlow subroutine with input $\underline{c}$. Let $d$ be the phase length return by MinFlow and define $t_{end} := t_{start}+d$. Then we have for any $h\in [H], s\in \cS_h, a \in \cA_h(s)$,
    \begin{align*}
        \overline{n}_h^{t_{end}}(s,a) - \overline{n}_h^{t_{start}}(s,a) \geq c_h(s,a).
    \end{align*}
\end{lemma}
